# Supplementary material for: Measuring Internet Routing from the Most Valuable Points
Source: arXiv:2405.13172 source file (2024-05-21)
Supplement: Supplementary file 1 [file appendix.tex]

\subsection{implementation}

In this section we will depict the implementation of our solution. The idea is to provide a free online
API (or make the server publicly available) where the user could do some requests. A request should
take the form of URL + load budget, and the user get the corresponding VP set, in a few seconds.

\myitem{The user do not need to recompute the graph features or the clusters.} Computing the graph features
is quite long. Indeed, to compute the graph features for the 500 events, it takes five days. This remain scalable
since the events are spread over three months, but leads to an useless overhead if a user needs to recompute them. This
is the main reason why we want to provide a centralized tool (with code publicly available). Our actual implementation
is done with scikit-learn and networkx packages and runs on a server with a i7 4.8 Ghz processor and 64 GB of RAM.

\subsection{tab with values}
